# Supplementary material for: Chiral twist drives raft formation and organization in membranes composed of rod-like particles
Source: arXiv:1608.07331 ancillary file (2016-10-31)
Supplement: Supplementary file 1 [file Supporting.pdf]

# Supporting Information: Chiral twist drives raft formation and organization in membranes composed of rod-like particles

Louis Kang[1,*] and T. C. Lubensky[1]

[1] *Department of Physics & Astronomy, University of Pennsylvania, 209 South 33rd Street, Philadelphia, Pennsylvania 19104, USA*

## CONTENTS

I. Derivation of the single-domain free energy 1

II. Calculation of the virus tilt angle 2

III. Calculation of the raft shift free energy 2

IV. Chiral contribution to phase separation 4

V. Landau coefficients for phase separation 5

VI. Overview of the linear system 7

VII. General membrane rafts formed from chiral rod-like particles 8

## I. DERIVATION OF THE SINGLE-DOMAIN FREE ENERGY

We must be careful to maintain volume conservation in this system, so let's conceptualize the raft formation process in two stages. First, the untwisted two-component membrane of radius $R_{\mathrm{t}}$ with raft area fraction $\alpha^2$ is divided into untwisted tiling domains of radius $R$ that each contains a raft of radius $\alpha R$ (Fig. 3b of the main text). Second, the rods in each domain twists with angle $\theta(r) \ll 1$ (Fig. 3c). Doing so, however, decreases the thickness of the membrane slightly, so to conserve volume in both the raft and the background, each domain has to grow slightly from radius $R$ to $R'$ and its raft must grow slightly from radius $\alpha R$ to $\alpha' R'$. Mathematically, volume conservation for the raft and the background appears respectively as

$$\int_0^{\alpha' R'} \mathrm{d}r\, r l_1 \cos\theta = \int_0^{\alpha R} \mathrm{d}r\, r l_1, \qquad \int_{\alpha' R'}^{R'} \mathrm{d}r\, r l_2 \cos\theta = \int_{\alpha R}^{R} \mathrm{d}r\, r l_2. \tag{S1}$$

If we expand to quadratic order in $\theta(r)$, we get

$$\int_0^{\alpha' R'} \mathrm{d}r\, r = \int_0^{\alpha R} \mathrm{d}r\, r + \frac{1}{2}\int_0^{\alpha' R'} \mathrm{d}r\, r\theta^2, \qquad \int_{\alpha' R'}^{R'} \mathrm{d}r\, r = \int_{\alpha R}^{R} \mathrm{d}r\, r + \frac{1}{2}\int_{\alpha' R'}^{R'} \mathrm{d}r\, r\theta^2. \tag{S2}$$

Thus, the projected areas in the $x$-$y$ plane of the raft and the background increase by terms proportional to $\theta^2$ due to rod twist and volume conservation (Fig. 3e).

The free energy of the raft and the background are each described by the single-component membrane free energies $F_{\mathrm{dep}}$ and $F_{\mathrm{Frank}}$ (Eqs. 1 and 7 of the main text). In addition, the change in membrane half-thickness by $d\cos\theta_0$ at the raft-background interface creates extra excluded volume, which leads to an interfacial line tension (Fig. 3d). The

* lkang@mail.med.upenn.edu

combination of these effects, to quadratic order in $\theta$ and the virus half-length difference $d$, gives

$$\frac{F_{\rm domain}}{4\pi caT} = d\alpha' R' + \int_0^{\alpha' R'} \mathrm{d}r \left[ r + \frac{\lambda_1^2}{2} \left( r(\partial_r\theta)^2 + 2\theta\partial_r\theta + \frac{\theta^2}{r} - 2q_1 r\partial_r\theta - 2q_1\theta \right) \right]$$
$$+ \int_{\alpha' R'}^{R'} \mathrm{d}r \left[ r + \frac{\lambda_2^2}{2} \left( r(\partial_r\theta)^2 + 2\theta\partial_r\theta + \frac{\theta^2}{r} - 2q_2 r\partial_r\theta - 2q_2\theta \right) \right]. \quad \text{(S3)}$$

$\lambda_j = \sqrt{K_j l_j / caT}$ is the twist penetration depth, where $j \in \{1, 2\}$ corresponds to raft and background, respectively. Actually, only the twist mode contributes to this free energy to quadratic order in $\theta$, so the single Frank elastic constant $K_j$ reflects only the twist elastic constant in this equation and does not correspond to the splay or bend elastic constants.

Using $2\theta\partial_r\theta = \partial_r(\theta^2)$, $r\partial_r\theta + \theta = \partial_r(r\theta)$, and Eqs. S2, the domain free energy becomes

$$\frac{F_{\rm domain}}{4\pi caT} = \frac{1}{2}R^2 + d\alpha' R' - \left[\lambda_1^2 q_1 - \lambda_2^2 q_2\right] \alpha' R' \theta_0 + \frac{1}{2}\left[\lambda_1^2 + \lambda_2^2\right]\theta_0^2$$
$$+ \int_0^{\alpha' R'} \mathrm{d}r \left[ \frac{1}{2} r\theta^2 + \frac{\lambda_1^2}{2}\left( r(\partial_r\theta)^2 + \frac{\theta^2}{r} \right) \right] + \int_{\alpha' R'}^{R'} \mathrm{d}r \left[ \frac{1}{2} r\theta^2 + \frac{\lambda_2^2}{2}\left( r(\partial_r\theta)^2 + \frac{\theta^2}{r} \right) \right]. \quad \text{(S4)}$$

Every term with $\alpha' R'$ and $R'$ is either linear or quadratic in $d$ and $\theta$, so to quadratic order, we can use $\alpha R$ and $R$ instead:

$$\frac{F_{\rm domain}}{4\pi caT} = \frac{1}{2}R^2 + d\alpha R - \left[\lambda_1^2 q_1 - \lambda_2^2 q_2\right] \alpha R \theta_0 + \frac{1}{2}\left[\lambda_1^2 + \lambda_2^2\right]\theta_0^2$$
$$+ \int_0^{\alpha R} \mathrm{d}r \left[ \frac{1}{2} r\theta^2 + \frac{\lambda_1^2}{2}\left( r(\partial_r\theta)^2 + \frac{\theta^2}{r} \right) \right] + \int_{\alpha R}^{R} \mathrm{d}r \left[ \frac{1}{2} r\theta^2 + \frac{\lambda_2^2}{2}\left( r(\partial_r\theta)^2 + \frac{\theta^2}{r} \right) \right]. \quad \text{(S5)}$$

To be precise, the radii $\alpha R$ and $R$ indicated in Fig. 3 of the main text should actually be their primed counterparts, but this correction is quadratic in $\theta$ and thus small. Multipling Eq. S5 by the number of rafts $R_{\rm t}^2/R^2$ gives the membrane structure free energy Eq. 9 of the main text, ignoring a constant term proportional to $R_{\rm t}^2$.

## II. CALCULATION OF THE VIRUS TILT ANGLE

From the membrane structure free energy Eq. 9 of the main text, we can calculate the virus tilt angle $\theta(r)$ by solving its Euler-Lagrange equations. We first focus on the raft domain and rewrite its integral in a dimensionless manner with the substitutions $s_1 = r/\lambda_1$ and $S_1 = R/\lambda_1$:

$$\int_0^{\alpha R} \mathrm{d}r \left[ \frac{1}{2} r\theta^2 + \frac{\lambda_1^2}{2}\left( r(\partial_r\theta)^2 + \frac{\theta^2}{r} \right) \right] = \frac{\lambda_1^2}{2}\int_0^{\alpha S_1} \mathrm{d}s_1 \left[ s_1\theta^2 + \frac{\theta^2}{s_1} + s_1(\partial_{s_1}\theta)^2 \right]$$
$$= \frac{\lambda_1^2}{2}\int_0^{\alpha S_1} \mathrm{d}s_1 \left[ s_1\theta\partial_{s_1}^2\theta + \theta\partial_{s_1}\theta + s_1(\partial_{s_1}\theta)^2 \right]$$
$$= \frac{\lambda_1^2}{2}\left( s_1\theta\partial_{s_1}\theta \right)\Big|_{s_1=0}^{\alpha S_1}, \quad \text{(S6)}$$

where the last two expressions were obtained through the Euler-Lagrange equation

$$s_1^2\partial_{s_1}^2\theta + s_1\partial_{s_1}\theta - (s_1^2 + 1)\theta = 0, \quad \text{(S7)}$$

which is a Bessel differential equation. The boundary conditions for the raft are $\theta(0) = 0$ and $\theta(\alpha S_1) = \theta_0$. We can obtain the same equation for the background with the substitutions $s_2 = r/\lambda_2$ and $S_2 = R/\lambda_2$, and its boundary conditions are $\theta(\alpha S_2) = \theta_0$ and $\theta(S_2) = 0$. Solving for $\theta(r)$ gives Eq. 11 of the main text.

## III. CALCULATION OF THE RAFT SHIFT FREE ENERGY

The shifted polar coordinates used to calculate the raft shift free energy are

$$x = r\cos\phi + b(r) \qquad \text{and} \qquad y = r\sin\phi. \quad \text{(S8)}$$

We calculate Eq. 18 of the main text explicitly by substituting in expressions for the scale factors

$$h_r = \sqrt{(\partial_r x)^2 + (\partial_r y)^2} = \sqrt{1 + 2\partial_r b \cos\phi + (\partial_r b)^2} \qquad \text{and} \qquad h_\phi = \sqrt{(\partial_\phi x)^2 + (\partial_\phi y)^2} = r \tag{S9}$$

and the nematic director

$$\mathbf{n}(r,\phi) = \sin\psi(r,\phi)\sin\theta(r,\phi)\,\hat{\mathbf{r}} - \cos\psi(r,\phi)\sin\theta(r,\phi)\,\hat{\boldsymbol{\phi}} + \cos\theta(r,\phi)\,\hat{\mathbf{z}}. \tag{S10}$$

$\theta(r,\phi) = \theta(r) + \vartheta(r)\cos\phi$, where $\theta$ and $\vartheta$ are the monopolar and dipolar components of the tilt angle. The angle $\psi(r,\phi) = \psi(r)\sin\phi$, also to dipolar order, rotates the tilt axis of the particles to produce an $\hat{\mathbf{r}}$ component in $\mathbf{n}$. The result, to quadratic order in the angles, is

$$\frac{F_{\text{shift}}}{2caT} = \int_{\alpha R}^{R} \mathrm{d}r \int_0^{2\pi} \mathrm{d}\phi \left\{ \frac{1}{2} r(\theta + \vartheta\cos\phi)^2 \sqrt{1 + 2\partial_r b\cos\phi + (\partial_r b)^2} + \frac{\lambda_2^2}{2} \frac{(r\partial_r\theta + r\partial_r\vartheta\cos\phi + \theta + \vartheta\cos\phi)^2}{r\sqrt{1 + 2\partial_r b\cos\phi + (\partial_r b)^2}} \right.$$
$$\left. + \frac{\lambda_2^2}{2} \frac{\left[\theta\partial_r b + \vartheta + 3\vartheta\partial_r b\cos\phi + \vartheta(\partial_r b)^2\right]^2 \sin^2\phi}{r\left[1 + 2\partial_r b\cos\phi + (\partial_r b)^2\right]^{3/2}} \right\}. \tag{S11}$$

Note that $\psi$ does not appear, so we set $\psi = 0$. The shifted coordinate system introduces splay deformations into this quadratic-order free energy, so the single Frank elastic constant describes the energetic cost of both twist and splay deformations. We can perfrom the integral over $\phi$ to obtain the complicated expression

$$\frac{F_{\text{shift}}}{2caT} = \int_{\alpha R}^{R} \frac{\mathrm{d}r}{r} \left\{ \frac{1}{1 + \partial_r b} k[\theta,\vartheta,b;r] K\left(\frac{2\sqrt{\partial_r b}}{1 + \partial_r b}\right) + (1 + \partial_r b) e[\theta,\vartheta,b;r] E\left(\frac{2\sqrt{\partial_r b}}{1 + \partial_r b}\right) \right\}, \tag{S12}$$

where $K$ and $E$ are complete elliptic integrals of the first and second kinds, respectively, and

$$k[\theta,\vartheta,b;r] = \lambda_2^2\theta^2\left[1 + (\partial_r b)^2\right] + 2\lambda_2^2(\theta + r\partial_r\theta)^2 - 2\lambda_2^2(\theta + r\partial_r\theta)(\vartheta + r\partial_r\vartheta)\left[1 + (\partial_r b)^2\right]$$
$$+ \frac{4}{3}(2r^2 + 3\lambda_2^2)\theta\vartheta\partial_r b - \frac{2}{3}(r^2 + \lambda_2^2)\frac{\theta\vartheta\left[1 + (\partial_r b)^2\right]}{\partial_r b} - \frac{1}{5}(2r^2 + 13\lambda_2^2)\vartheta^2\left[1 + (\partial_r b)^2\right]$$
$$+ \frac{1}{15}(r^2 + 9\lambda_2^2)\frac{\vartheta^2\left[1 + (\partial_r b)^2\right]\left[1 + 4(\partial_r b)^2 + (\partial_r b)^4\right]}{(\partial_r b)^2} + \frac{1}{3}\lambda_2^2\frac{(\vartheta + r\partial_r\vartheta)^2\left[1 + 4(\partial_r b)^2 + (\partial_r b)^4\right]}{(\partial_r b)^2} \tag{S13}$$

$$e[\theta,\vartheta,b;r] = (2r^2 - \lambda_2^2)\theta^2 + \frac{2}{3}(r^2 + 3\lambda_2^2)\frac{\theta\vartheta\left[1 + (\partial_r b)^2\right]}{\partial_r b} + 2\lambda_2^2\frac{(\theta + r\partial_r\theta)(\vartheta + r\partial_r\vartheta)}{\partial_r b}$$
$$+ \frac{1}{3}(4r^2 + 9\lambda_2^2)\vartheta^2 - \frac{1}{15}(r^2 + 9\lambda_2^2)\frac{\vartheta^2\left[1 + 4(\partial_r b)^2 + (\partial_r b)^4\right]}{(\partial_r b)^2} - \frac{1}{3}\lambda_2^2\frac{(\vartheta + r\partial_r\vartheta)^2\left[1 + (\partial_r b^2)\right]}{(\partial_r b)^2}. \tag{S14}$$

We can simplify the shift energy Eq. S12 in the limit of small raft shifts with $\partial_r b \ll 1$. Assuming small deformations, we expect that $\theta$ retains its unshifted profile (Eq. 11 of the main text). We can directly calculate $\Delta F_{\text{shift}}$, which is $F_{\text{shift}}$ minus the unshifted free energy of the domain in which $b = 0$. To quadratic order in $\partial_r b$,

$$\frac{\Delta F_{\text{shift}}}{4\pi caT} = \int_{\alpha R}^{R} \mathrm{d}r \left\{ \frac{1}{8}\left[2r\vartheta^2 + r\theta^2(\partial_r b)^2\right] + \frac{\lambda_2^2}{8}\left[2r(\partial_r\vartheta)^2 + 4\vartheta\partial_r\vartheta + 4\frac{\vartheta^2}{r} + \left(r(\partial_r\theta)^2 + 2\theta\partial_r\theta + 3\frac{\theta^2}{r}\right)(\partial_r b)^2\right]\right\}. \tag{S15}$$

First, note that $\vartheta$ and $b$ are uncoupled. The terms corresponding to $\vartheta$ can be written as a sum of squares, so $\vartheta = 0$. Thus,

$$\frac{\Delta F_{\text{shift}}}{4\pi caT} = \int_{\alpha R}^{R} \mathrm{d}r \left[\frac{1}{8}r\theta^2 + \frac{\lambda_2^2}{8}\left(r(\partial_r\theta)^2 + 2\theta\partial_r\theta + 3\frac{\theta^2}{r}\right)\right](\partial_r b)^2. \tag{S16}$$

In the large radius limit where $\alpha R \gg \lambda_2$, we can make numerous simplifications, including

$$\theta(r) \sim \theta_0\sqrt{\frac{\alpha R}{r}}\frac{\sinh[(R - r)/\lambda_2]}{\sinh[(R - \alpha R)/\lambda_2]}. \tag{S17}$$

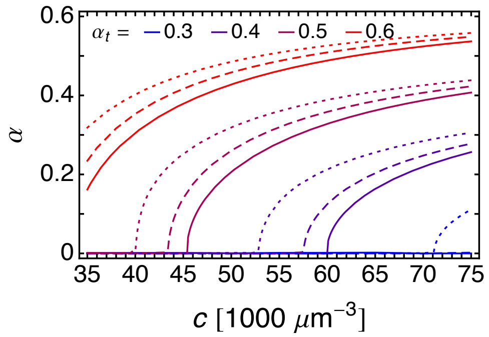


FIG. S1. Phase separation using a total free energy incorporating raft structure and organization. $\alpha^2$ is the area fraction of the raft phase, and it is obtained by numerically minimizing the sum of Eqs. 4 and 13 of the main text over a range of depletant concentrations $c$. We use the same parameter values given in Table I of the main text, except that the chiral wavenumbers $q_{fd}$ and $q_{\mathrm{M13}}$ are multipled by a factor of 1 (solid), 2 (dashed), or 2.5 (dotted). The solid lines are indistinguishable from Fig. 2d of the main text, which plots Eq. 5 As the chiral wavenumber difference increases in magnitude past a critical value, $\alpha$ increases beyond its value in Eq. 5 and phase separation begins at lower values of $c$.

This transforms Eq. S16 to

$$\frac{\Delta F_{\mathrm{shift}}}{4\pi caT} = \frac{\alpha R}{8}\operatorname{csch}^2\left[(R-\alpha R)/\lambda_2\right]\theta_0^2\int_{\alpha R}^{R}\mathrm{d}r\cosh\left[2(R-r)/\lambda_2\right](\partial_r b)^2. \tag{S18}$$

The Euler-Lagrange equation for $b(r)$ can be integrated to give

$$b(r) \approx b_0\frac{\arctan\tanh[(R-r)/\lambda_2]}{\arctan\tanh[(R-\alpha R)/\lambda_2]}. \tag{S19}$$

Substituting this into Eq. S18 yields the energy

$$\frac{\Delta F_{\mathrm{shift}}}{4\pi caT} \approx \frac{\alpha R}{8\lambda_2}\frac{\operatorname{csch}^2[(R-\alpha R)/\lambda_2]}{\arctan\tanh[(R-\alpha R)/\lambda_2]}\theta_0^2 b_0^2. \tag{S20}$$

## IV. CHIRAL CONTRIBUTION TO PHASE SEPARATION

With the parameter values given in Table I of the main text, numerical minimization of the total free energy combining bare phase separation (Eq. 4) and raft structure (Eq. 13) over $\alpha$ and $R$ yields results indistingushable from sequential minimization of Eq. 4 over $\alpha$ and Eq. 13 over $R$. However, after multiplying both chiral wavenumbers $q_{fd}$ and $q_{\mathrm{M13}}$ by various factors, combined minimization and sequential minimization produce different results (Fig. S1). Note that Eq. 4 does not depend on $\Delta q$ and the Frank constant $K$, whereas Eq. 13 does. Thus, increasing the magnitude of the chiral wavenumber difference $\Delta q$ places the system in a regime where the chiral membrane structure influences the degree of phase separation. A larger $|\Delta q|$ leads to a larger $\alpha$, facilitating phase separation.

We can see this effect of $\Delta q$ on $\alpha$ analytically in the $R \to \infty$ limit, where Eq. 13 becomes Eq. 14 of the main text. We introduce a small correction $\Delta\alpha$ that the structural free energy imposes on the $\alpha$ preferred by the phase separation free energy (Eq. 5 of the main text):

$$\alpha = \sqrt{\frac{\alpha_{\mathrm{t}}^2 - \mathrm{e}^{-2cd/c_{\mathrm{v}}}}{1-\mathrm{e}^{-2cd/c_{\mathrm{v}}}}} + \Delta\alpha. \tag{S21}$$

We then expand the combined free energy (Eq. 4 plus Eq. 14) to leading orders in $\Delta\alpha$ and $1/R$:

$$\frac{F_{\mathrm{sep}}+F_{\mathrm{struct}}}{\pi R_{\mathrm{t}}^2 T} = \frac{F^0_{\mathrm{sep}}+F^0_{\mathrm{struct}}}{\pi R_{\mathrm{t}}^2 T} + 4c\frac{a}{R}\left(d - \frac{1}{4}\lambda^3\Delta q^2\right)\Delta\alpha + c_{\mathrm{v}}\frac{(\alpha_{\mathrm{t}}^2 - \mathrm{e}^{-2cd/c_{\mathrm{v}}})(1-\mathrm{e}^{-2cd/c_{\mathrm{v}}})}{(1-\alpha_{\mathrm{t}}^2)\mathrm{e}^{-2cd/c_{\mathrm{v}}}}\Delta\alpha^2. \tag{S22}$$

Here, the 0 superscript indicates the unperturbed free energies that do not depend on $\Delta\alpha$. The coefficient of the

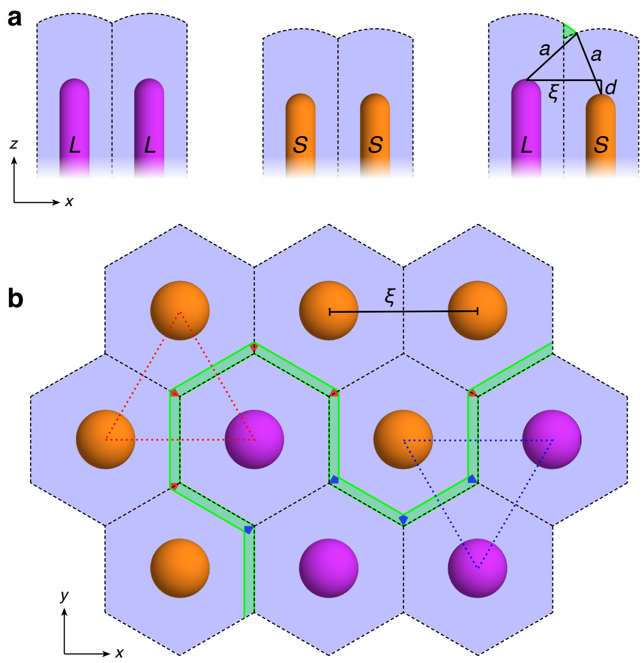


FIG. S2. An Ising-like model for depletion-induced phase separation in the limit of small virus half-length difference $d$. **a**, A membrane composed of longer $L$ viruses (left) contains more excluded volume per particle (blue) than a membrane composed of shorter $S$ viruses (middle), which leads to a linear term in the Ising-like Hamiltonian Eq. S23. A virus pair consisting of one $L$ and one $S$ particle (right) occupies more excluded volume than the average of a pair of two $L$ particles and a pair of two $S$ particles. This extra excluded volume (green) has approximate cross-sectional area $ad^2/2\xi$ and leads to quadratic terms in Eq. S23. **b**, Assuming a hexagonal lattice of viruses, a nearest-neighbor triplet consisting of one $L$ virus and two $S$ viruses (red dotted triangle, for example) produces slightly more excluded volume than a triplet consisting of two $L$ viruses and one $S$ virus (blue dotted triangle, for example). These small additions (dark red regions) and reductions (dark blue regions) in excluded volume contribute cubic terms in Eq. S23. Schematics not drawn to scale.

quadratic term is always positive when $\alpha \neq 0$. The coefficient of the linear term includes an overall factor of $a/R$ and is thus small for large $R$. When it is positive, the membrane is in the regime of a single large raft, so $R \to \infty$ and the linear term vanishes. The membrane thus prefers $\Delta\alpha = 0$, and the structure of the membrane does not affect phase separation. The coefficient of the linear term changes sign at the transition from a single large raft to multiple smaller rafts, becoming negative in the latter regime and favoring a positive $\Delta\alpha$. Thus, we directly see in this limit that $F_{\text{sep}}$ dominates the behavior of $\alpha$ and that chirality facilitates phase separation, since a larger $|\Delta q|$ favors a larger $\Delta\alpha$.

## V. LANDAU COEFFICIENTS FOR PHASE SEPARATION

In the main text, we argued that mixing preferentially occurs in the background phase and can be ignored in the raft phase because a long rod among a sea of short ones contributes much more extra excluded volume than a short rod among a sea of long ones (Fig. 2c of the main text). However, if we imagine decreasing the difference in virus half-lengths $d$ to a very small value, excluded volume differences should be severely reduced and mixing should occur in both phases. Here, we explore the onset of phase separation and asymmetric mixing properties in the limit $d \ll \xi/2 \ll a$, where $\xi$ is the virus-virus separation and $a$ is the depletant radius. Note that the first inequality is not compatible with the experimental values $d = 130\,\text{nm}$ and $\xi = 12\,\text{nm}$ used in the main text.

The membrane can be described by an Ising-like model in this limit. We assume a hexagonal lattice with lattice constant $\xi$ whose sites are occupied with either a long $L$ virus or a short $S$ virus. $L$ viruses naturally contribute more excluded volume—$\sqrt{3}\xi^2 d$ per particle—than do the $S$ viruses. However, because of the effect of surface convexity on excluded volume, an $L$ particle will contribute an even greater amount of excluded volume when it is adjacent to an $S$ particle (Fig. S2a)—approximately $ad^2/\sqrt{3}$ per $L$-$S$ pair. And since this extra excluded volume lies closer to the $S$ virus in each heterogeneous pair, a symmetry between $L$ and $S$ viruses is broken, and three-particle couplings are permitted. Indeed, as depicted in Fig. S2b, there are even smaller amounts of additional and reduced excluded volume for $L$-$S$-$S$ and $L$-$L$-$S$ nearest-neighbor triplets, respectively—approximately $\pm\pi a^2 d^3/9\xi^2$ per triplet. Using Eq. 1 of

the main text, we can write these excluded volume effects in terms of a depletion free energy. We use $\phi_{\mathbf{i}}^L \in \{0,1\}$ to indicate the absence and presence, respectively, of an $L$ particle at lattice site $\mathbf{i}$; $\phi_{\mathbf{i}}^S = 1 - \phi_{\mathbf{i}}^L$ acts similarly as an indicator for $S$ viruses. The effective Ising-like Hamiltonian is

$$\begin{aligned}\frac{H}{Tc} &= \sqrt{3}\xi^2 d \sum_{\mathbf{i}} \phi_{\mathbf{i}}^L + \frac{1}{\sqrt{3}} a d^2 \sum_{\langle \mathbf{ij} \rangle} \left( \phi_{\mathbf{i}}^L \phi_{\mathbf{j}}^S + \phi_{\mathbf{i}}^S \phi_{\mathbf{j}}^L \right) \\ &\quad + \frac{\pi}{9} \frac{a^2 d^3}{\xi^2} \sum_{\langle \mathbf{ijk} \rangle} \left[ \left( \phi_{\mathbf{i}}^L \phi_{\mathbf{j}}^S \phi_{\mathbf{k}}^S + \phi_{\mathbf{i}}^S \phi_{\mathbf{j}}^L \phi_{\mathbf{k}}^S + \phi_{\mathbf{i}}^S \phi_{\mathbf{j}}^S \phi_{\mathbf{k}}^L \right) - \left( \phi_{\mathbf{i}}^L \phi_{\mathbf{j}}^L \phi_{\mathbf{k}}^S + \phi_{\mathbf{i}}^L \phi_{\mathbf{j}}^S \phi_{\mathbf{k}}^L + \phi_{\mathbf{i}}^S \phi_{\mathbf{j}}^L \phi_{\mathbf{k}}^L \right) \right], \end{aligned} \tag{S23}$$

where $\langle \mathbf{ij} \rangle$ indicates nearest-neighbor pairs of lattice sites and $\langle \mathbf{ijk} \rangle$ indicates nearest-neighbor triplets of lattice sites. $c$ is depletant concentration and $T$ is temperature. We convert the $\phi$'s to the symmetric order parameter $\psi_{\mathbf{i}} = \pm 1$, where positive (negative) corresponds to an $L$ ($S$) virus at site $\mathbf{i}$. Thus,

$$\phi_{\mathbf{i}}^L = \frac{1+\psi_{\mathbf{i}}}{2} \qquad \text{and} \qquad \phi_{\mathbf{i}}^S = \frac{1-\psi_{\mathbf{i}}}{2}. \tag{S24}$$

This converts Eq. S23 to

$$\frac{H}{Tc} = \frac{\sqrt{3}}{2}\xi^2 d \sum_{\mathbf{i}} \psi_{\mathbf{i}} - \frac{1}{2\sqrt{3}} a d^2 \sum_{\langle \mathbf{ij} \rangle} \psi_{\mathbf{i}} \psi_{\mathbf{j}} + \frac{\pi}{12} \frac{a^2 d^3}{\xi^2} \sum_{\langle \mathbf{ijk} \rangle} \psi_{\mathbf{i}} \psi_{\mathbf{j}} \psi_{\mathbf{k}}, \tag{S25}$$

to leading orders in $d$ and ignoring constant terms.

The first term acts as a chemical potential that would favor $\psi_{\mathbf{i}} = -1$; for our system, we assume that the membrane, once formed, maintains fixed numbers of $L$ and $S$ viruses. Thus, $\sum_{\mathbf{i}} \psi_{\mathbf{i}}$ is conserved and we ignore the linear term. We now take mean-field and continuum limits. For the quadratic term, we allow slow variations in the mean-field order parameter $\psi(x,y) \equiv \langle \psi_{\mathbf{i}} \rangle$, which reflects the local concentration difference between the two virus species, with

$$\begin{aligned}\sum_{\langle \mathbf{ij} \rangle} \psi_{\mathbf{i}} \psi_{\mathbf{j}} &\to c_{\mathrm{v}} \int \mathrm{d}x\,\mathrm{d}y\,\psi(x,y) \left[ \psi(x-\xi,y) + \psi\left( x + \frac{\xi}{2}, y + \frac{\sqrt{3}\xi}{2} \right) + \psi\left( x + \frac{\xi}{2}, y - \frac{\sqrt{3}\xi}{2} \right) \right] \\ &= c_{\mathrm{v}} \int \mathrm{d}x\,\mathrm{d}y \left[ 3\psi(x,y)^2 + \frac{3}{4}\xi^2 \psi(x,y)(\partial_x^2 + \partial_y^2)\psi(x,y) \right] \\ &= c_{\mathrm{v}} \int \mathrm{d}^2\mathbf{x} \left[ 3\psi^2 - \frac{3}{4}\xi^2 (\boldsymbol{\nabla}\psi)^2 \right], \end{aligned} \tag{S26}$$

where we have integrated by parts and ignored boundary terms. $c_{\mathrm{v}} = 2/\sqrt{3}\xi^2$ is the 2D virus concentration. For the cubic term, we notice that there are twice as many nearest-neighbor triplets as lattice points to obtain

$$\sum_{\langle \mathbf{ijk} \rangle} \psi_{\mathbf{i}} \psi_{\mathbf{j}} \psi_{\mathbf{k}} \to 2c_{\mathrm{v}} \int \mathrm{d}^2\mathbf{x}\,\psi^3. \tag{S27}$$

The mean-field Hamiltonian is thus (without the linear term)

$$\frac{\langle H \rangle}{c_{\mathrm{v}} T} = c a d^2 \int \mathrm{d}^2\mathbf{x} \left[ -\frac{\sqrt{3}}{2}\psi^2 + \frac{\pi}{6}\frac{ad}{\xi^2}\psi^3 + \frac{\sqrt{3}}{8}\xi^2 (\boldsymbol{\nabla}\psi)^2 \right]. \tag{S28}$$

Meanwhile, the entropy of mixing follows in analogy to Eq. 3 of the main text with the substitutions in Eq. S24:

$$\frac{S_{\mathrm{mix}}}{c_{\mathrm{v}}} = \int \mathrm{d}^2\mathbf{x} \left[ \frac{1-\psi}{2} \log \frac{1-\psi}{2} + \frac{1+\psi}{2} \log \frac{1+\psi}{2} \right]. \tag{S29}$$

Thus, the free energy to leading orders in $\psi$ is

$$\frac{F_{\mathrm{Landau}}}{c_{\mathrm{v}} T} = \frac{\langle H \rangle - T S_{\mathrm{mix}}}{c_{\mathrm{v}} T} = \int \mathrm{d}^2\mathbf{x} \left[ \left( \frac{1}{2} - \frac{\sqrt{3}}{2} c a d^2 \right) \psi^2 + \frac{\pi}{6} \frac{c a^2 d^3}{\xi^2} \psi^3 + \frac{1}{12}\psi^4 + \frac{\sqrt{3}}{8} c a d^2 \xi^2 (\boldsymbol{\nabla}\psi)^2 \right]. \tag{S30}$$

This expression provides values for the coefficients of a phenomenological Landau expansion in $\psi$, such as that used in Ref. [39] of the main text. It illustrates the equivalence between our system and liquid-gas phase separation, with a critical point at $c = 1/\sqrt{3}ad^2$. Around this point, $cad^2 \sim 1$, so the characteristic domain wall width between regions of different $\psi$'s is the interparticle distance $\sim\xi$. When $c$ exceeds this critical value, the free energy Eq. S30 has both positive and negative local minima:

$$\psi_\pm = \pm\sqrt{\frac{1}{\sqrt{3}}cad^2 - \frac{1}{3}} - \frac{\pi}{12}\frac{ca^2d^3}{\xi^2} \tag{S31}$$

to leading orders in $d$. Note that the cubic term, which arises from asymmetric effects of depletion on long versus short particles, makes $\psi_+$ less positive and $\psi_-$ more negative, indicating that mixing is enhanced in the $L$-rich phase and hindered in the $S$-rich phase. As $d$ increases, these effects grow until the $S$-rich phase can be considered completely pure and all mixing occurs in $L$-rich phase, a regime demonstrated by the raft and background phases of *fd* and M13 viruses in the main text.

## VI. OVERVIEW OF THE LINEAR SYSTEM

Here we present the major results of a rectangular membrane whose rafts are arranged as linear stripes of wavelength $2L$. Note that the same results can be obtained by taking the $R \to \infty$ limit of the circular raft system. The membrane has dimensions $L_x$ and $L_y$, and the nematic director describing particle orientation is $\mathbf{n}(x) = -\sin\theta(x)\hat{\mathbf{y}} + \cos\theta(x)\hat{\mathbf{z}}$. The membrane free energy, in analogy to Eq. 9 of the main text, is

$$\frac{F_{\text{linear}}}{2caTL_y} = \frac{L_x}{L}\left\{d - \left[\lambda_1^2 q_1 - \lambda_2^2 q_2\right]\theta_0 + \int_0^{\alpha L}\mathrm{d}x\left[\frac{1}{2}\theta^2 + \frac{\lambda_1^2}{2}(\partial_x\theta)^2\right] + \int_{\alpha L}^{L}\mathrm{d}x\left[\frac{1}{2}\theta^2 + \frac{\lambda_2^2}{2}(\partial_x\theta)^2\right]\right\}. \tag{S32}$$

The $q$'s and $\lambda$'s are defined identically to their definitions in the main text, with the raft phase extending from 0 to $\alpha L$ and the background phase from $\alpha L$ to $L$. The Euler-Lagrange equations for the raft and background phases are simply $\lambda_j^2\partial_x^2\theta - \theta = 0$, with $j \in \{1, 2\}$. The boundary conditions are $\theta(0) = 0$, $\theta(\alpha L) = \theta_0$, and $\theta(L) = 0$. Thus,

$$\theta(x) = \begin{cases} \theta_0 \dfrac{\sinh(x/\lambda_1)}{\sinh(\alpha L/\lambda_1)} & 0 < x < \alpha L \\ \theta_0 \dfrac{\sinh[(L-x)/\lambda_2]}{\sinh[(L-\alpha L)/\lambda_2)]} & \alpha L < x < L. \end{cases} \tag{S33}$$

Substituting this into Eq. S32 yields

$$\frac{F_{\text{linear}}}{2caTL_y} = \frac{L_x}{L}\left\{d - \left[\lambda_1^2 q_1 - \lambda_2^2 q_2\right]\theta_0 + \frac{1}{2}\Big[\lambda_1\coth(\alpha L/\lambda_1) + \lambda_2\coth[(L-\alpha L)/\lambda_2]\Big]\theta_0^2\right\}. \tag{S34}$$

Thus,

$$\theta_0 = \frac{\lambda_1^2 q_1 - \lambda_2^2 q_2}{\lambda_1\coth(\alpha L/\lambda_1) + \lambda_2\coth[(L-\alpha L)/\lambda_2]}, \tag{S35}$$

leading to

$$\frac{F_{\text{linear}}}{2caTL_y} = \frac{L_x}{L}\left\{d - \frac{1}{2}\frac{\left[\lambda_1^2 q_1 - \lambda_2^2 q_2\right]^2}{\lambda_1\coth(\alpha L/\lambda_1) + \lambda_2\coth[(L-\alpha L)/\lambda_2]}\right\} \tag{S36}$$

$$= \frac{L_x}{L}\left\{d - \frac{1}{2}\frac{\lambda^3\Delta q^2}{\coth(\alpha L/\lambda) + \coth[(L-\alpha L)/\lambda]}\right\}, \tag{S37}$$

under the assumption that $\lambda \equiv \lambda_1 = \lambda_2$, where $\Delta q = q_1 - q_2$.

In the limit where $L \to \infty$, this becomes

$$\frac{F_{\text{linear}}}{2caTL_y} \sim \frac{L_x}{L}\left\{d - \frac{1}{4}\lambda^3\Delta q^2 + \frac{1}{4}\lambda^3\Delta q^2\left[\mathrm{e}^{-2\alpha L/\lambda} + \mathrm{e}^{-2(1-\alpha)L/\lambda}\right]\right\}. \tag{S38}$$

Unlike the circularly-symmetric case, there are no higher-order polynomial terms in $L^{-1}$. Thus, the transition to finite-sized striped rafts is directly analogous to the 1D Frenkel-Kontorova model at the commensurate-incommensurate transition.

We believe that the free-floating experimental system adopts a circular geometry due to the energy of the membrane edge, which, due to depletion, prefers rods to be tilted along the tangent to the edge. Perhaps a linear, striped configuration can be seen in very large or spherical membranes where edge effects are not important.

## VII. GENERAL MEMBRANE RAFTS FORMED FROM CHIRAL ROD-LIKE PARTICLES

Our theory easily generalizes to any membrane raft system that has three properties. First, the membrane particles are chiral and rod-like, and thus prefer to twist at a particular wavenumber. This is described by the chiral Frank free energy presented as Eq. 7 of the main text, with single elastic constant $K$ and chiral wavenumber $q$. Second, the particles prefer to align perpendicular to the membrane. This appears to lowest order as a harmonic free energy

$$F_{\text{align}} = \frac{D}{2} \int \mathrm{d}^2\mathbf{x}\, \theta^2. \tag{S39}$$

$D$ is analogous to the smectic liquid crystal alignment parameter, but it multiplies an integral over 2D, not 3D, space. Third, a line tension exists at the interfaces between the two phases:

$$F_{\text{tension}} = \gamma \int_C \mathrm{d}s, \tag{S40}$$

where the line integral travels along all interfaces $C$.

We approximate the rafts to tile the circular membrane of radius $R_{\text{t}}$ via circular domains of radius $R$, just as in Fig. 3 of the main text. We take the raft area fraction $\alpha^2$ to be an experimental parameter, though for certain systems, it may be possible to determine $\alpha$ from more fundamental physical principles, in analogy to the entropically-derived Eq. 4. The structural free energy of this generalized system is

$$\frac{F_{\text{gen}}}{2\pi} = \frac{R_{\text{t}}^2}{R^2}\Bigg\{\gamma\alpha R - [K_1 t_1 q_1 - K_2 t_2 q_2]\,\alpha R \theta_0 + \frac{1}{2}[K_1 t_1 + K_2 t_2]\,\theta_0^2 + \int_0^{\alpha R} \mathrm{d}r \left[\frac{D_1}{2} r\theta^2 + \frac{K_1 t_1}{2}\left(r(\partial_r\theta)^2 + \frac{\theta^2}{r}\right)\right] + \int_{\alpha R}^{R} \mathrm{d}r \left[\frac{D_2}{2} r\theta^2 + \frac{K_2 t_2}{2}\left(r(\partial_r\theta)^2 + \frac{\theta^2}{r}\right)\right]\Bigg\} \tag{S41}$$

$t$ is the thickness of the membrane, and the subscripts 1 and 2 refer to raft and background phases respectively. Reference [39] of the main text arrives at a similar free energy, but the differences in parameter values between raft and background phases in their work arise from a two-species Landau theory in terms of the area fraction of one of the virus species.

Minimizing $F_{\text{gen}}$ with respect to $\theta$ and then $\theta_0$ proceeds analogously to the virus case. With the boundary conditions $\theta(0) = 0$, $\theta(\alpha R) = \theta_0$, and $\theta(R) = 0$:

$$\theta(r) = \begin{cases} \theta_0 \dfrac{I_1(s_1)}{I_1(\alpha S_1)} & 0 \le r \le \alpha R \\ \theta_0 \dfrac{K_1(s_2)/K_1(S_2) - I_1(s_2)/I_1(S_2)}{K_1(\alpha S_2)/K_1(S_2) - I_1(\alpha S_2)/I_1(S_2)} & \alpha R \le r \le R, \end{cases} \tag{S42}$$

where $I_\nu$ and $K_\nu$ are modified Bessel functions of the first and second kind, respectively, of order $\nu$. To prevent confusion of the latter for Frank constants, we define $k_j \equiv K_j t_j$, for $j \in \{1, 2\}$, as an effective 2D Frank elastic constant, where $K_j$ refers to the 3D Frank constant. The twist penetration depths are $\lambda_j \equiv \sqrt{k_j/D_j}$, which rescale the distances as $s_j = r/\lambda_j$ and $S_j = R/\lambda_j$. The maximum twist angle is

$$\theta_0 = \frac{k_1 q_1 - k_2 q_2}{\sqrt{D_1 k_1}\frac{I_0(\alpha S_1)}{I_1(\alpha S_1)} + \sqrt{D_2 k_2}\frac{K_0(\alpha S_2)/K_1(S_2) + I_0(\alpha S_2)/I_1(S_2)}{K_1(\alpha S_2)/K_1(S_2) - I_1(\alpha S_2)/I_1(S_2)}}. \tag{S43}$$

After integrating out $\theta$, $F_{\text{gen}}$ becomes

$$\frac{F_{\text{struct}}}{2\pi R_{\text{t}}^2} = \frac{\alpha}{R}\left\{\gamma - \frac{1}{2}\frac{(k_1 q_1 - k_2 q_2)^2}{\sqrt{D_1 k_1}\frac{I_0(\alpha S_1)}{I_1(\alpha S_1)} + \sqrt{D_2 k_2}\frac{K_0(\alpha S_2)/K_1(S_2)+I_0(\alpha S_2)/I_1(S_2)}{K_1(\alpha S_2)/K_1(S_2)-I_1(\alpha S_2)/I_1(S_2)}}\right\}, \tag{S44}$$

a major result of the main text, but here for generalized membranes.
